# Supplementary material for: Closing the gap between atomic-scale lattice deformations and continuum elasticity
Source: arXiv:1808.05190 source file (2019-04-24)
Supplement: Supplementary file 1 [file SupportingInformation.pdf]

# *Supporting Information for:*
# Closing the gap between atomic-scale lattice deformations and continuum elasticity

Marco Salvalaglio,[1,*] Axel Voigt,[1,2] and Ken Elder[3]
[1] *Institute of Scientific Computing, Technische Universität Dresden, 01062 Dresden, Germany*
[2] *Dresden Center for Computational Materials Science (DCMS), TU Dresden, 01062 Dresden, Germany*
[3] *Department of Physics, Oakland University, Rochester, 48309 Michigan, USA.*

## S1. RECIPROCAL SPACE VECTORS FOR DIFFERENT SYMMETRIES

In the APFC approach the crystal lattice symmetry is fixed by considering a proper set of $N$ vectors $\mathbf{k}_j$. For triangular symmetry $N = 3$ and reciprocal-space vectors are

$$\mathbf{k}_1 = k_0\left(-\sqrt{3}/2, -1/2\right) \qquad \mathbf{k}_2 = k_0(0,1) \qquad \mathbf{k}_3 = k_0\left(\sqrt{3}/2, -1/2\right) \tag{S1}$$

with $k_0 = 1$. For bcc symmetry $N = 6$ and the reciprocal-space vectors are

$$\begin{aligned} \mathbf{k}_1 = k_0\,(1,1,0)\,, \qquad \mathbf{k}_2 = k_0\,(1,0,1)\,, \qquad \mathbf{k}_3 = k_0\,(0,1,1)\,, \\ \mathbf{k}_4 = k_0\,(0,1,-1)\,, \qquad \mathbf{k}_5 = k_0\,(1,-1,0)\,, \qquad \mathbf{k}_6 = k_0\,(-1,0,1)\,. \end{aligned} \tag{S2}$$

with $k_0 = \sqrt{2}/2$. For fcc symmetry $N = 7$ and the reciprocal-space vectors are

$$\begin{aligned} \mathbf{k}_1 = k_0\,(-1,1,1)\,, \qquad \mathbf{k}_2 = k_0\,(1,-1,1)\,, \qquad \mathbf{k}_3 = k_0\,(1,1,-1)\,, \qquad \mathbf{k}_4 = k_0\,(-1,-1,-1)\,, \\ \mathbf{k}_5 = k_0\,(2,0,0)\,, \qquad \mathbf{k}_6 = k_0\,(0,2,0)\,, \qquad \mathbf{k}_7 = k_0\,(0,0,2)\,. \end{aligned} \tag{S3}$$

with $k_0 = \sqrt{3}/3$.

## S2. STRAIN-FIELD AND ROTATION-FIELD COMPONENTS FROM AMPLITUDES

In the main text, the derivation of the displacement field $\mathbf{u}$ and, in turn, of the strain $\boldsymbol{\varepsilon}$ and rotation $\boldsymbol{\omega}$ tensors is discussed. The result is that they are functions of $\mathbf{k}_j$ vectors and $\partial\varphi_j/\partial x_i$ with $\varphi_j = \arctan\left[\mathrm{Im}(\eta_j)/\mathrm{Re}(\eta_j)\right]$.

For 2D systems, the components of $\boldsymbol{\varepsilon}$ are given by

$$\begin{aligned} \varepsilon_{xx} &= \frac{1}{\mathbf{k}_l \times \mathbf{k}_m}\left[k_m^y \frac{\partial\varphi_l}{\partial x} - k_l^y \frac{\partial\varphi_m}{\partial x}\right] \\ \varepsilon_{yy} &= \frac{1}{\mathbf{k}_l \times \mathbf{k}_m}\left[k_l^x \frac{\partial\varphi_m}{\partial y} - k_m^x \frac{\partial\varphi_l}{\partial y}\right] \\ \varepsilon_{xy} &= \frac{1}{2\mathbf{k}_l \times \mathbf{k}_m}\left[k_m^y \frac{\partial\varphi_l}{\partial y} - k_l^y \frac{\partial\varphi_m}{\partial y} + k_l^x \frac{\partial\varphi_m}{\partial x} - k_m^x \frac{\partial\varphi_l}{\partial x}\right] \end{aligned} \tag{S4}$$

with $l$ and $m$ label different amplitudes as in (3) in the main text. Analogously, $\omega$ is given by

$$\omega = \frac{1}{2\mathbf{k}_l \times \mathbf{k}_m}\left[k_m^y \frac{\partial\varphi_l}{\partial y} - k_l^y \frac{\partial\varphi_m}{\partial y} - k_l^x \frac{\partial\varphi_m}{\partial x} + k_m^x \frac{\partial\varphi_l}{\partial x}\right] \tag{S5}$$

*Electronic address: marco.salvalaglio@tu-dresden.de

For 3D systems, $\varepsilon_{ij}$ are given by

$$
\begin{aligned}
\varepsilon_{xx} &= \frac{1}{\mathbf{k}_n\cdot(\mathbf{k}_m\times\mathbf{k}_l)}\left[\frac{\partial\varphi_l}{\partial x}\left(k_m^z k_n^y - k_m^y k_n^z\right) + \frac{\partial\varphi_m}{\partial x}\left(k_n^z k_l^y - k_n^y k_l^z\right) + \frac{\partial\varphi_n}{\partial x}\left(k_l^z k_m^y - k_l^y k_m^z\right)\right]\\
\varepsilon_{yy} &= \frac{1}{\mathbf{k}_n\cdot(\mathbf{k}_m\times\mathbf{k}_l)}\left[\frac{\partial\varphi_l}{\partial y}\left(k_m^x k_n^z - k_m^z k_n^x\right) + \frac{\partial\varphi_m}{\partial y}\left(k_n^x k_l^z - k_n^z k_l^x\right) + \frac{\partial\varphi_n}{\partial y}\left(k_l^x k_m^z - k_l^z k_m^x\right)\right]\\
\varepsilon_{zz} &= \frac{1}{\mathbf{k}_n\cdot(\mathbf{k}_m\times\mathbf{k}_l)}\left[\frac{\partial\varphi_l}{\partial z}\left(k_m^y k_n^x - k_m^x k_n^y\right) + \frac{\partial\varphi_m}{\partial z}\left(k_n^y k_l^x - k_n^x k_l^y\right) + \frac{\partial\varphi_n}{\partial z}\left(k_l^y k_m^x - k_l^x k_m^y\right)\right]\\
\varepsilon_{xy} &= \frac{1}{2\mathbf{k}_n\cdot(\mathbf{k}_m\times\mathbf{k}_l)}\left[\frac{\partial\varphi_l}{\partial y}\left(k_m^z k_n^y - k_m^y k_n^z\right) + \frac{\partial\varphi_m}{\partial y}\left(k_n^z k_l^y - k_n^y k_l^z\right) + \frac{\partial\varphi_n}{\partial y}\left(k_l^z k_m^y - k_l^y k_m^z\right)\right]+\\
&+\frac{1}{2\mathbf{k}_n\cdot(\mathbf{k}_m\times\mathbf{k}_l)}\left[\frac{\partial\varphi_l}{\partial x}\left(k_m^x k_n^z - k_m^z k_n^x\right) + \frac{\partial\varphi_m}{\partial x}\left(k_n^x k_l^z - k_n^z k_l^x\right) + \frac{\partial\varphi_n}{\partial x}\left(k_l^x k_m^z - k_l^z k_m^x\right)\right]\\
\varepsilon_{xz} &= \frac{1}{2\mathbf{k}_n\cdot(\mathbf{k}_m\times\mathbf{k}_l)}\left[\frac{\partial\varphi_l}{\partial z}\left(k_m^z k_n^y - k_m^y k_n^z\right) + \frac{\partial\varphi_m}{\partial z}\left(k_n^z k_l^y - k_n^y k_l^z\right) + \frac{\partial\varphi_n}{\partial z}\left(k_l^z k_m^y - k_l^y k_m^z\right)\right]+\\
&+\frac{1}{2\mathbf{k}_n\cdot(\mathbf{k}_m\times\mathbf{k}_l)}\left[\frac{\partial\varphi_l}{\partial x}\left(k_m^y k_n^x - k_m^x k_n^y\right) + \frac{\partial\varphi_m}{\partial x}\left(k_n^y k_l^x - k_n^x k_l^y\right) + \frac{\partial\varphi_n}{\partial x}\left(k_l^y k_m^x - k_l^x k_m^y\right)\right]\\
\varepsilon_{yz} &= \frac{1}{2\mathbf{k}_n\cdot(\mathbf{k}_m\times\mathbf{k}_l)}\left[\frac{\partial\varphi_l}{\partial z}\left(k_m^x k_n^z - k_m^z k_n^x\right) + \frac{\partial\varphi_m}{\partial z}\left(k_n^x k_l^z - k_n^z k_l^x\right) + \frac{\partial\varphi_n}{\partial z}\left(k_l^x k_m^z - k_l^z k_m^x\right)\right]+\\
&+\frac{1}{2\mathbf{k}_n\cdot(\mathbf{k}_m\times\mathbf{k}_l)}\left[\frac{\partial\varphi_l}{\partial y}\left(k_m^y k_n^x - k_m^x k_n^y\right) + \frac{\partial\varphi_m}{\partial y}\left(k_n^y k_l^x - k_n^x k_l^y\right) + \frac{\partial\varphi_n}{\partial y}\left(k_l^y k_m^x - k_l^x k_m^y\right)\right]
\end{aligned}
\tag{S6}
$$

with $l$,$m$ and $n$ label different amplitudes as in (4) in the main text. The components of $\boldsymbol{\omega}$ in 3D are

$$
\begin{aligned}
\omega_{xy} &= \frac{1}{2\mathbf{k}_n\cdot(\mathbf{k}_m\times\mathbf{k}_l)}\left[\frac{\partial\varphi_l}{\partial y}\left(k_m^z k_n^y - k_m^y k_n^z\right) + \frac{\partial\varphi_m}{\partial y}\left(k_n^z k_l^y - k_n^y k_l^z\right) + \frac{\partial\varphi_n}{\partial y}\left(k_l^z k_m^y - k_l^y k_m^z\right)\right]-\\
&-\frac{1}{2\mathbf{k}_n\cdot(\mathbf{k}_m\times\mathbf{k}_l)}\left[\frac{\partial\varphi_l}{\partial x}\left(k_m^x k_n^z - k_m^z k_n^x\right) + \frac{\partial\varphi_m}{\partial x}\left(k_n^x k_l^z - k_n^z k_l^x\right) + \frac{\partial\varphi_n}{\partial x}\left(k_l^x k_m^z - k_l^z k_m^x\right)\right]\\
\omega_{xz} &= \frac{1}{2\mathbf{k}_n\cdot(\mathbf{k}_m\times\mathbf{k}_l)}\left[\frac{\partial\varphi_l}{\partial z}\left(k_m^z k_n^y - k_m^y k_n^z\right) + \frac{\partial\varphi_m}{\partial z}\left(k_n^z k_l^y - k_n^y k_l^z\right) + \frac{\partial\varphi_n}{\partial z}\left(k_l^z k_m^y - k_l^y k_m^z\right)\right]-\\
&-\frac{1}{2\mathbf{k}_n\cdot(\mathbf{k}_m\times\mathbf{k}_l)}\left[\frac{\partial\varphi_l}{\partial x}\left(k_m^y k_n^x - k_m^x k_n^y\right) + \frac{\partial\varphi_m}{\partial x}\left(k_n^y k_l^x - k_n^x k_l^y\right) + \frac{\partial\varphi_n}{\partial x}\left(k_l^y k_m^x - k_l^x k_m^y\right)\right]\\
\omega_{yz} &= \frac{1}{2\mathbf{k}_n\cdot(\mathbf{k}_m\times\mathbf{k}_l)}\left[\frac{\partial\varphi_l}{\partial z}\left(k_m^x k_n^z - k_m^z k_n^x\right) + \frac{\partial\varphi_m}{\partial z}\left(k_n^x k_l^z - k_n^z k_l^x\right) + \frac{\partial\varphi_n}{\partial z}\left(k_l^x k_m^z - k_l^z k_m^x\right)\right]-\\
&-\frac{1}{2\mathbf{k}_n\cdot(\mathbf{k}_m\times\mathbf{k}_l)}\left[\frac{\partial\varphi_l}{\partial y}\left(k_m^y k_n^x - k_m^x k_n^y\right) + \frac{\partial\varphi_m}{\partial y}\left(k_n^y k_l^x - k_n^x k_l^y\right) + \frac{\partial\varphi_n}{\partial y}\left(k_l^y k_m^x - k_l^x k_m^y\right)\right]
\end{aligned}
\tag{S7}
$$

## S3. 2D MULTILAYER: STRAIN-FIELD COMPONENTS

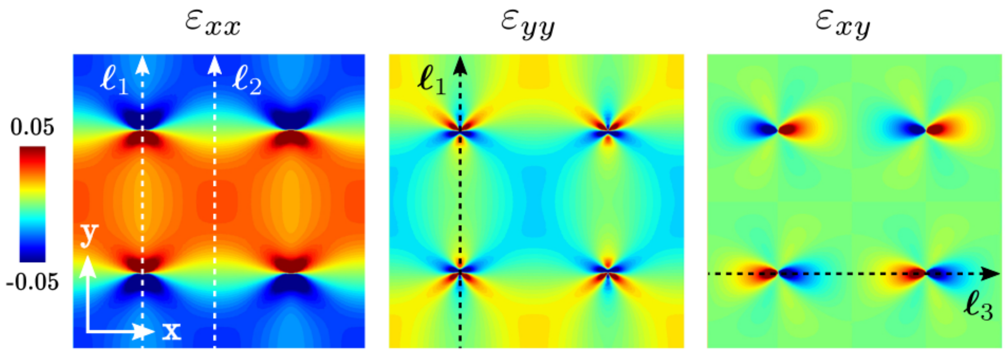


FIG. S1: Strain field components for the 2D multilayer system illustrated in Fig. 1 in the main text. They are computed from $\eta_j$ with $l = 1$ and $m = 2$.

In Fig. 1, the strain field is illustrated as a two-dimensional color map in terms of $\varepsilon_{xx}$ only, while comparisons with the elastic field computed from continuous elasticity (see also Sec. S4) are shown for all the components of $\boldsymbol{\varepsilon}$. Fig. S1 shows all the strain components of such a system. Moreover, it also shows the directions $\ell_i$ along which the elastic fields are compared in Fig. 1.

## S4. DISLOCATION ELASTIC FIELD FROM CONTINUUM ELASTICITY THEORY

The elastic field of a dislocation can be described by continuum elasticity theory, provided that the dislocation character, namely edge, screw or mixed [i], as well as the Burgers vector $\mathbf{b}$ are known. For $d = 2$, the Burgers vector as in Fig. 1(c) is actually intrinsically perpendicular to the ideal dislocation line, that is, in turn, perpendicular to the two-dimensional domain. Therefore, dislocations observed therein have edge character. The analytic stress field $\boldsymbol{\sigma}^{\rm d}$ of an edge dislocation with core in $\mathbf{x}_c = (0, 0)$ and $\mathbf{b}$ aligned to the $\mathbf{x}$ axis is here considered [i]. In order to remove the singularity inherently present at the dislocation core different approaches can be used [ii, iii]. Here, we use the regularization introduced in Ref. [iii] is considered (and here reported in the assumption of infinite, straight dislocation). The stress field components read

$$
\begin{aligned}
\sigma_{xx}/\sigma_0 &= -y\left(3\zeta^2 + 3x^2 + y^2\right), \\
\sigma_{yy}/\sigma_0 &= -y\left(\zeta^2 - x^2 + y^2\right), \\
\sigma_{zz}/\sigma_0 &= -2\nu y\left(2\zeta^2 + x^2 + y^2\right), \\
\sigma_{xy}/\sigma_0 &= x\left(\zeta^2 + x^2 - y^2\right) \\
\sigma_{xz} &= \sigma_{yz} = 0
\end{aligned}
\tag{S8}
$$

with

$$
\sigma_0 = \frac{E|\mathbf{b}|}{4\pi(1-\nu^2)\left(\zeta^2 + x^2 + y^2\right)^2}, \tag{S9}
$$

$E$ the Young modulus, and $\nu$ the Poisson ratio. $\zeta$ is the parameter controlling the regularization of the elastic field at the core, here arbitrarily set to $\zeta = |\mathbf{b}|/2$. The system illustrated in Fig. 1 consists of a portion of an infinite 2D array of dislocations, as imposed by PBC, with the same Burgers vector when moving along the interface between layers, and opposite when moving in the direction perpendicular to the interface (see also the orientation of dislocations in Fig. 1). The total stress field, $\boldsymbol{\sigma}^{\rm tot}$ is then obtained by superposing the field $\boldsymbol{\sigma}^{\rm d}$ originated from each defect in such an array, accounting for the proper orientation of $\mathbf{b}$ and a proper shift of $\mathbf{x}_c$. The strain field is computed by exploiting Hooke's law, i.e.,

$$
\boldsymbol{\varepsilon}^{\rm ce} = [(1+\nu)/E]\boldsymbol{\sigma}^{\rm tot} - (\nu/E){\rm tr}(\boldsymbol{\sigma}^{\rm tot})\mathbf{I} \tag{S10}
$$

Notice that, from (S8), $\boldsymbol{\sigma}^{\mathrm{d}} \propto E$, so that the only constant to be defined is $\nu$ set to 1/3 [iv, v].

---

[i] P.M. Anderson, J.P. Hirth, and J. Lothe. Theory of Dislocations. Cambridge University Press, 2017.
[ii] M. Lazar, G. A. Maugin Int. J. of Engineering Science **43**, 1157 (2005)
[iii] W Cai, A Arsenlis, C Weinberger, and V Bulatov. J. Mech. Phys. Solids, **54**, 561 (2006).
[iv] K. R. Elder, Mark Katakowski, Mikko Haataja, and Martin Grant. Phys. Rev. Lett. **88**, 245701 (2002).
[v] K. R. Elder and Martin Grant. Phys. Rev. E **70**, 051605 (2004).
